# Supplementary material for: Greedy-Based Feature Selection for Efficient LiDAR SLAM
Source: arXiv:2103.13090 source file (2021-03-24)
Supplement: Supplementary file 1 [file appendix.tex]

\appendix
%This appendix contains additional details in this paper.
\subsection{Expressions of Jacobians}
\label{app.jacobian_initialization}

\subsubsection{Planar Residuals}
The residuals in \eqref{equ.objective_initialization} are rewritten as:
\begin{equation}
\begin{aligned}
\mathbf{r}
\triangleq
\mathbf{r}_{\mathcal{F}}(\mathbf{x},\mathbf{p}) 	
&=
\big[
\mathbf{w}^{\top}(\mathbf{R}\mathbf{p}+\mathbf{t}) + d
\big]
\mathbf{w}\\
&=
\text{diag}(\mathbf{w})
\begin{bmatrix}
\mathbf{w}^{\top}\\
\mathbf{w}^{\top}\\
\mathbf{w}^{\top}
\end{bmatrix}
(\mathbf{R}\mathbf{p}+\mathbf{t})
+d\mathbf{w}\\
&=
\mathbf{A}_{\mathbf{w}}(\mathbf{R}\mathbf{p}+\mathbf{t})+d\mathbf{w}.
\end{aligned}	
\end{equation}

Using  $\mathbf{R}(\theta+\delta\theta)\approx\mathbf{R}(\mathbf{I}+\delta\theta^{\wedge})$, the Jacobians of the rotation are calculated as:
\begin{equation}
\label{equ.residual_jacobian_rotation}
\begin{aligned}
\frac{\partial \mathbf{r}}{\partial\mathbf{R}}
=
-\mathbf{A}_{\mathbf{w}}\mathbf{R}\mathbf{p}^{\wedge}.
\end{aligned}
\end{equation}

The Jacobians of the translation are
\begin{equation}
\label{equ.residual_jacobian_translation}
\begin{aligned}
\frac{\partial \mathbf{r}}{\partial\mathbf{t}}
=
\mathbf{A}_{\mathbf{w}}.
\end{aligned}
\end{equation}

\subsubsection{Optimization With Online Calibration}
The objective function in \eqref{equ.objective_online_calibration} has two terms: $f_{\mathcal{M}}(\mathcal{X}_{v})$ and $f_{\mathcal{M}}(\mathcal{X}_{e})$. For the first term, the Jacobians are given by
\begin{equation}
\begin{aligned}
%	\frac{\partial \mathbf{r}}{\partial\mathbf{R}_{p}}
%	&=
%	-\mathbf{A}\mathbf{R}_{p}^{\top}(\mathbf{R}_{K}\mathbf{p}+\mathbf{t}_{K}-\mathbf{t}_{p})^{\wedge}\\
%	\frac{\partial \mathbf{r}}{\partial\mathbf{t}_{p}}
%	&=
%	-\mathbf{A}\mathbf{R}_{p}^{\top}\\
\frac{\partial f_{\mathcal{M}}}{\partial\mathbf{R}_{K}}
&=
-\mathbf{A}_{\mathbf{w}}\mathbf{R}_{p}^{\top}\mathbf{R}_{K}\mathbf{p}^{\wedge},\\
\frac{\partial f_{\mathcal{M}}}{\partial\mathbf{t}_{K}}
&=
-\mathbf{A}_{\mathbf{w}}\mathbf{R}_{p}^{\top},
\end{aligned}
\end{equation}
where $	k \in [p+1, N+1]$.
Since the second term has the same form as \eqref{equ.objective_initialization}, the Jacobians are given by \eqref{equ.residual_jacobian_rotation} and \eqref{equ.residual_jacobian_translation} as:
\begin{equation}
\begin{aligned}
\frac{\partial f_{\mathcal{M}}}{\partial\mathbf{R}_{l^{i}}^{b}}
&=
-\mathbf{A}_{\mathbf{w}}\mathbf{R}_{l^{i}}^{b}\mathbf{p}^{\wedge},\\
\frac{\partial f_{\mathcal{M}}}{\partial\mathbf{t}_{l^{i}}^{b}}
&=
-\mathbf{A}_{\mathbf{w}},
\end{aligned}
\end{equation}
where $i\in[2, I]$.

\subsubsection{Optimization With Pure Odometry}
Moreover, the Jacobians of the residuals in \eqref{equ.objective_pure_odometry} are computed as:
\begin{equation}
\begin{aligned}
\frac{\partial f_{\mathcal{M}}}{\partial\mathbf{R}_{K}}
&=
-\mathbf{A}_{\mathbf{w}}\mathbf{R}_{p}^{\top}\mathbf{R}_{K}(\mathbf{R}_{l^{i}}^{b}\mathbf{p}+\mathbf{t}_{l^{i}}^{b})^{\wedge},\\	
\frac{\partial f_{\mathcal{M}}}{\partial\mathbf{t}_{K}}
&=
-\mathbf{A}_{\mathbf{w}}\mathbf{R}_{p}^{\top},\\	
\end{aligned}
\end{equation}
where $i \in [1, I]$ and $k \in [p+1, N+1]$.
